# Supplementary material for: Smooth Non-Rigid Shape Matching via Effective Dirichlet Energy Optimization
Source: arXiv:2210.02870 source file (2022-10-05)
Supplement: Supplementary file 1 [file appendix_smooth.tex]

Here we review 
\subsection{nICP: Non-Rigid ICP}
Non-rigid ICP~\cite{nicp} proposes a surface registration method to wrap the source shape $\Ss_1$ to the target shape $\Ss_2$, such that the wrapped $\Ss_1$ is close to the target shape (via a distance energy), and the deformations are locally rigid (via a stiffness energy). An extra term of landmark preservation is added if pre-specified landmarks are provided.
Specifically, nICP models the deformation as an affine transformation at each vertex,  i.e., a $3\times 4$ matrix $D_i$ at vertex $v_i$ in homogeneous coordinates $(x_i, y_i, z_i, 1)^T$. Therefore, after applying the affine transformation at each vertex, we get the new vertex positions $D_i v_i$.

The smoothness of the deformation field $\*D$ on $\Ss_2$ (dimension $n_2\times 3 \times 4$) is controlled via the graph Laplacian of the shape which we note $\Delta_2$. The total energy (up to some dropped correspondences and a landmarks term) is
\begin{equation}\label{eq:smooth:nicp}
    E_{\text{nICP}}(\Pi_{21}, D) = \big\Vert D\big\Vert_{\Delta_2}^2 + \al \big\Vert \Pi_{21} X_1 - D X_2\big\Vert^2_F
\end{equation}

This energy can be seen as a derivation of the minimization of the \emph{graph} Dirichlet energy $\Vert \Pi_{21} X_1\Vert_{\Delta_2}^2$, where some quadratic splitting was done by setting $D$ so that $D X_2 \simeq \Pi_{21} X_1$ with $D$ affine at each vertex. The second term of Eq.~\eqref{eq:smooth:nicp} can now be seen as a coupling term, while the first one is the now transformed energy.
\\
The minimization for each variable leads to a linear system and a nearest neighbor search.

\subsection{APAP:As-Rigid-As Possible}
ARAP~\cite{arap} proposes the following energy to formulate locally rigid deformations on a shape $S$:
\begin{equation}\label{eq:smooth:arap}
    E_{\text{ARAP}}(R_i, p') = \sum_{(p_i, p_j)\in\mathcal{E}(S)} w_{ij} \big\Vert \inpar{p'_i - p'_j} - R_i \inpar{p_i-p_j} \big\Vert_2^2,
\end{equation}

where $p$ is the vertex coordinate in the original shape $\Ss$, $p'$ is the corresponding new position in the deformed shape $\Ss'$, and $R_i$ is a rotation matrix defined on the $i$-th vertex to enforce the local rigidity between $\Ss$ and $\Ss'$.

We can rewrite ARAP energy via Dirichlet energies. Specifically, we denote the original and the deformed shape as $\Ss_1$ and $\Ss_2$ respectively with the correspondences $\Pi_{21}$ from $\Ss_2$ to $\Ss_1$. Therefore, $\Pi_{21}X_1$ gives the new positions of the deformed shapes. By expanding Eq.~\eqref{eq:smooth:arap}, we get
\begin{equation}
    \begin{split}
    E_{\text{arap}}(\Pi_{21}, R) &= \big\Vert \Pi_{21} X_1\big\Vert^2_{W_1} + \big\Vert X_1\big\Vert^2_{W_1} - 2 \big\langle\,\Pi_{21} X_1, B(R) X_2\,\big\rangle \\
    \end{split}
\end{equation}
with $\big(B(R)X_2\big)_i = \sum_{j\in\Nn(i)} w_{ij} \big(R_i+R_j\big)\big(X_i-X_j\big)$. \jing{something wrong.}
%We recognize the dirichlet energy and a second term ensuring the computed correspondences fit the design choice.  Note that in the case, we solve directly for $\Pi_{21}X_1$ and don't apply quadratic splitting. Solving reduces to closed form solution for $R$ and linear system for $\Pi_{21}X_1$.

\subsection{RHM: Reversible Harmonic Maps}
\cite{RHM}

\subsection{Smooth Shells}
\cite{smoothshells}
